# Supplementary material for: Differential Dynamic Programming for Multi-Phase Rigid Contact Dynamics
Source: arXiv:1904.05072 source file (2019-04-10)
Supplement: Supplementary file 1 [file appendix.tex]

\section*{Appendix}

Appendixes should appear before the acknowledgment.
